# Supplementary material for: Community Detection Guarantees Using Embeddings Learned by Node2Vec
Source: arXiv:2310.17712 source file (2024-10-22)
Supplement: Supplementary file 1 [file minima.tex]

\subsection{Properties of minima}

TODO list:
\begin{itemize}
    \item split this into three: parts a) and b) of the lemma, proving
    that the minima is of low rank, and part c) - separate into different
    sections
    \item figure out the low rank of the minima stuff
    \item finish off the proof of part c)
\end{itemize}

Recall that we have earlier defined 
\begin{equation}
    \mcR_n(U, V) := \frac{1}{n^2} \sum_{i, j \in [n]}
    \Big\{  
        - \psamphat \rho_n W(\lambda_u, \lambda_v) \log(\sigma(\embedip)) 
        - \nsamphat \log(1 - \sigma(\embedip))
    \Big\}.
\end{equation}

\begin{lemma}
    Define the modified function
    \begin{equation}
        \mcR_n(M) := \frac{1}{n^2} \sum_{i, j \in [n]}
        \Big\{  
            - \psamphat \rho_n W(\lambda_u, \lambda_v) \log(\sigma(M_{ij})) 
            - \nsamphat \log(1 - \sigma(M_{ij}))
        \Big\}.
    \end{equation}
    over all matrices $M \in \mathbb{R}^{n \times n}$. Then we have
    the following:
    \begin{enumerate}[label=\alph*)]
        \item The function $\mcR_n(M)$ is strictly convex in $M$.
        \item The global minimizer of $\mcR_n(M)$ is given by
        \begin{equation}
            M^*_{ij} = \log\Big(  \frac{ 
                \psamphat \rho_n W(\lambda_i, \lambda_j)  }{   \nsamphat   }     \Big)
        \end{equation}
        and satisfies $\nabla_M \mcR_n(M) = 0$. 
        \item We have the lower bound
        \begin{equation}
            \mcR_n(M) - \mcR_n(M^*) \geq c \cdot
            \Big( 232 \Big)
        \end{equation}
        which holds for $c = 232$.
    \end{enumerate}
\end{lemma}

\begin{proof}
    For part a), this follows by the fact that the functions
    $-\log(\sigma(x))$ and $-\log(1 - \sigma(x))$ are positive
    and strictly convex functions of $x \in \mathbb{R}$, the fact
    that $\psamphat \rho_n W(\lambda_i, \lambda_j)$ and
    $\nsamphat$ are positive quantities which are 
    bounded above (see e.g
    Lemma~\ref{app:thm:add_diag}), and the fact that the sum of
    strictly convex functions is strictly convex. 
    
    For part b),
    this follows by noting that each of the $M_{ij}^*$ are pointwise
    minima of the functions
    \begin{equation}
        r_{ij}(x) =  - \psamphat \rho_n W(\lambda_u, \lambda_v) \log(\sigma(x))) 
        - \nsamphat \log(1 - \sigma(x))
    \end{equation}
    defined over $x \in \mathbb{R}$. Indeed, note that
    \begin{equation}
        \frac{d r_{ij}}{dx} =  (-1 + \sigma(x)) \psamphat \rho_n W(\lambda_u, \lambda_v) 
        + \sigma(x) \nsamphat,
    \end{equation}
    so setting this equal to zero, rearranging and making use of the
    equality $\sigma^{-1}(a/(a+b)) = \log(a/b)$ gives the stated result.

    For part c), we again make use of the individual functions
    $r_{ij}$ to obtain lower bounds. 
    To do so, note that by the integral versions of Taylor's theorem,
    for a twice different function $f$ one has for all $x, y \in \mathbb{R}$ that 
    \begin{align}
        f(x) = f(y) + f'(y)(x-y) + \int_0^1 (1-t) f''(tx + (1-t)y) (x - y)^2 \, dt.
    \end{align}
    Applying this to $f(x) = - \log \sigma(x)$ gives 
    \begin{equation}
        -\log\sigma(x) = -\log\sigma(y) + (-1 + \sigma(y))(x-y) + \int_0^1
        (1 - t) 
    \end{equation}
\end{proof}

Substituting in the values for $\psamphat$ and $\nsamphat$ gives
\begin{align}
    M_{ij}^* = & \log\Big( \frac{ 2 P_{c(i), c(j)} \mcE_W(\alpha)}{    
        (1 + k^{-1}) \mathbb{E}[\theta] \mathbb{E}[\theta]^{\alpha} \big( 
        \theta_j^{\alpha - 1} \widetilde{P}_{c(i)} 
        \widetilde{P}_{c(j)}^{\alpha}
            + \theta_i^{\alpha - 1} \widetilde{P}_{c(i)}^{\alpha} 
            \widetilde{P}_{c(j)}
            \big) }   \Big) \\
    = & \log\Big( \frac{ 2 \mcE_W(\alpha) }{ 
        (1 + k^{-1}) \mathbb{E}[\theta] \mathbb{E}[\theta]^{\alpha} } \Big) 
    + \log\Big( \frac{  P_{c(i), c(j)} }{ 
        \widetilde{P}_{c(i)} \widetilde{P}_{c(j)}   
        \cdot \big(   
            \theta_i^{\alpha - 1} \widetilde{P}_{c(i)}^{\alpha - 1}
        + \theta_j^{\alpha - 1} \widetilde{P}_{c(j)}^{\alpha - 1}
        \big)}   \Big) 
    \\ 
    =& \log\Big( \frac{ 2 \mcE_W(\alpha) }{ 
        (1 + k^{-1}) \mathbb{E}[\theta] \mathbb{E}[\theta]^{\alpha} } \Big) 
    + \log\Big( \frac{  P_{c(i), c(j)} }{ 
        \widetilde{P}_{c(i)} \widetilde{P}_{c(j)}   
        }   \Big) 
        - \log\Big( \theta_i^{\alpha - 1} \widetilde{P}_{c(i)}^{\alpha - 1}
        + \theta_j^{\alpha - 1} \widetilde{P}_{c(j)}^{\alpha - 1} \Big)
\end{align}
We now prove some useful properties about the matrix $M^*$.

\begin{lemma}
    232
\end{lemma}

\begin{lemma}
    Suppose that $A, B \in \mathbb{R}^{n \times n}$ are matrices, and
    $B_{ij} \neq 0$ for all $i, j$. Then if $\rk(B) = 1$, it follows that the
    matrices
    \begin{equation}
        (A \circ B)_{ij} := A_{ij} B_{ij}, \qquad
        (A / B)_{ij} := A_{ij} / B_{ij}
    \end{equation}
    have rank equal to $\rk(A)$. 
\end{lemma}

\begin{proof}
    We first note that for $A, B \in \mathbb{R}^{n \times n}$, the rank
    of the Hadamard product $A \circ B$ satisfies
    \begin{equation}
        \rk(A \circ B) \leq \rk(A) \cdot \rk(B).
    \end{equation}
    If we define $(A / B)_{ij} = A_{ij} / B_{ij}$ where $B_{ij} \neq 0$ for all $i, j$, 
    then a consequence
    of the above inequality applied to the fact that $A = (A / B) \circ B$ is that
    \begin{equation}
        \rk(A) / \rk(B) \leq \rk(A / B).
    \end{equation}
    Now, suppose that $B_{ij}$ is a rank one matrix, so $B_{ij} = u_i v_j$ for
    two vectors $u, v \in \mathbb{R}^n$. Provided $u_i \neq 0$ and $v_j \neq 0$ for all
    $i$, we can write $(1/B)_{ij} = (1/u_i) \cdot (1/v_j)$, and so $(1/B)$ is also
    a matrix of rank $1$. In particular, as we can write $A \circ B = A / (1 /B)$, 
    we have that
    \begin{equation}
        \rk(A) \leq \rk(A / (1/B)) = \rk(A \circ B) \leq \rk(A),
    \end{equation}
    meaning we have equality throughout. The same argument applies for $A / B$ by
    noting that $A / B = A \circ (1/B)$. 
\end{proof}

\begin{lemma}

\end{lemma}
